# Supplementary material for: Modelling repetition in zDM: a single population of repeating fast radio bursts can explain CHIME data
Source: arXiv:2306.17403 source file (2023-09-18)
Supplement: Supplementary file 1 [file excluded_appendix.tex]

\section{On the applicability of the DM selection function}
\label{sec:modelling_systematics}

In \secref{sec:CHIME}, we have used the published CHIME selection function, $s({\rm DM})$, to model CHIME's DM-dependent bias. We then find a small systematic difference between CHIME observations and the predictions of the \zdm\ code when using the best-fit parameters of \cite{Shin2022}. A possible explanation was posited as being due to differences in the modelling. Here we elaborate on that difference.

Within the \zdm\ code, the underlying FRB population is treated as having a distribution of widths \citep[with scattering now being explicitly modelled][]{James2022_H0}. However, spectral structure is not modelled, and FRBs are characterised by their properties at band centre. The CHIME/FRB experiment uses a wide fractional bandwidth of 50\%, and its search algorithm weights either towards high or low frequencies \citep{chime_injection_2022}. Therefore, in \citet{CHIME_catalog1_2021}, the authors develop a model for the FRB population which includes this spectral structure, and the CHIME/FRB's system response to it is estimated by a pulse injection method \citep{chime_injection_2022}. The DM selection function, $s({\rm DM})$, is averaged over this distribution, weighted by the modelled intrinsic population. This intrinsic FRB population has different properties to that assumed by the \zdm\ code --- for instance, the intrinsic width distribution used in \zdm\ is wider \citep{James2022_H0} --- and this will result in a different DM efficiency function even for the same actual system response. Without knowing what the underlying, multi-dimensional source FRB population is, it is impossible to know to what degree $s({\rm DM})$ reflects the system response, and to what extent the source population. 

\subsection{Efficiency function}

\begin{figure}
    \centering
\includegraphics[width=0.49\textwidth]{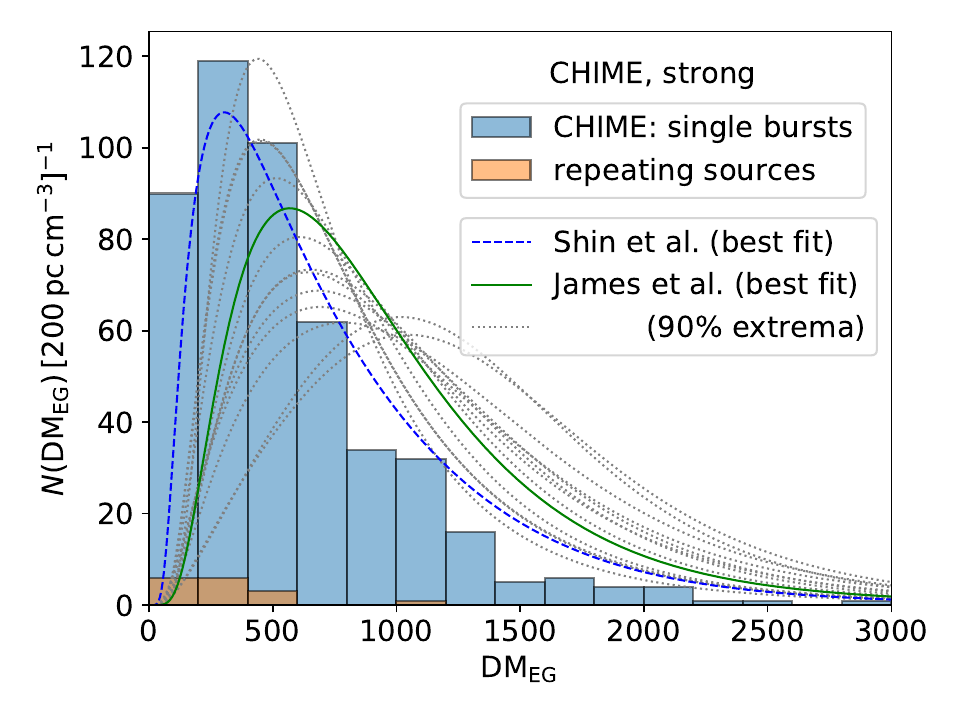}\\
\includegraphics[width=0.49\textwidth]{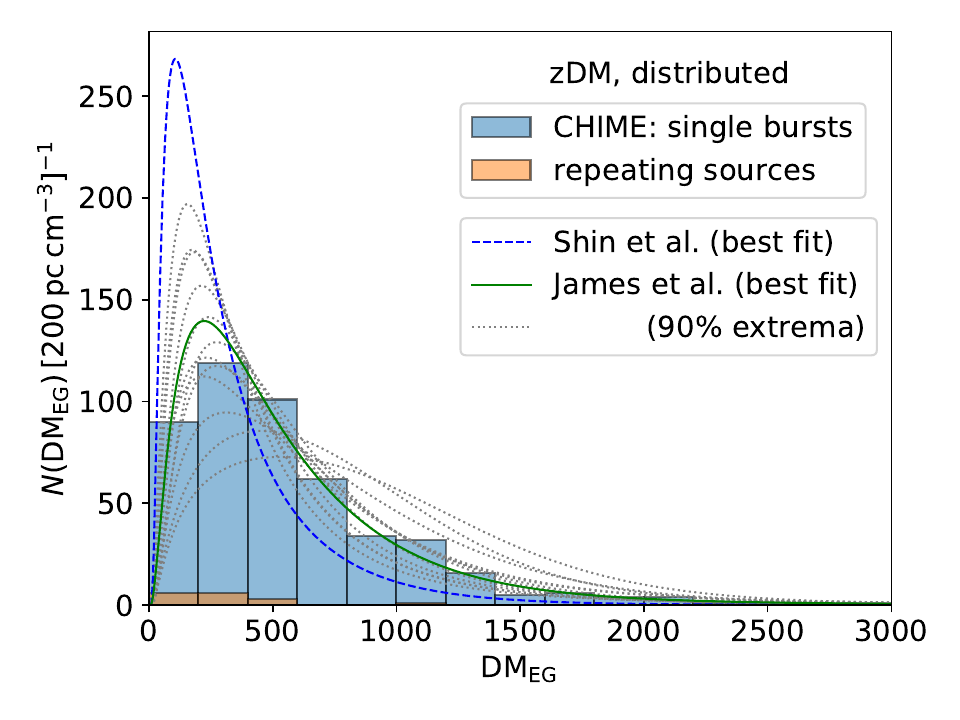}
    \caption{Observed rates of CHIME FRBs, showing sources observed as single and repeating, summed over declination. These are compared to estimates for the number of single bursts using the best-fit results from \citet{Shin2022} (solid, blue) and \citet{James2022_H0} (dashed, green), and 90\% extreme (dotted, grey) values of population parameters from Table~\ref{tab:pop_params}, with DM bias estimated using only the time--frequency resolution of the instrument, and assuming a population of repeating FRBs with `distributed' (top) and `strong' (bottom) repetition rates. Predicted singles rates are normalised to observed singles rates.}
    \label{fig:example_chime_decs}
\end{figure}

We also consider the {\sc zdm} efficiency function from \figref{fig:chime_dm_bias}. This is not to say that this function is more justifiable than that published by \citet{CHIME_catalog1_2021}. However, such an efficiency function is inevitably defined relative to some initial assumed FRB population. Thus the efficiency functions of \citet{CHIME_catalog1_2021} and \citet{James2022Meth} would be a better fits to the intrinsic FRB populations assumed in those works, and since we use the methods/population of the latter, we consider the latter's efficiency functions.

The result is shown in Figure~\ref{fig:example_chime_decs} (right). For distributed repeaters, the \jh\ (p=0.76), min \emax\ (p=0.011), max $\gamma$ (p=0.70), and min \sigmahost\ (p=0.015) scenarios are broadly compatible, while for strong repeaters, \jh\ (p=0.06), \emax\ (p=0.11), and max $\gamma$ (p=0.10) scenarios are compatible at the 1\% level or greater. The total number of FRBs are here under-predicted however, with predictions ranging from 42--221 against 505 observed. Reducing the FRB threshold to between 0.95 and 2.9\,Jy\,ms would approximately account for this difference. This is also more plausible, since we expect this efficiency function to apply to lower thresholds.
